# Supplementary material for: When-To-Post on Social Networks
Source: arXiv:1506.02089 source file (2015-06-05)
Supplement: Supplementary file 1 [file igt073d-spasojevic_appendix.tex]

\newpage
\afterpage{\null\newpage}

\newpage
\afterpage{\null\newpage}

\newpage
\newpage

\begin{table*}[htbp]
\caption{Twitter Followers}
\begin{center}
\begin{tabular}{|l|c|c|c|c|c|c|c|}
\hline
row & 0 & 1 & 2 & 3 & 4 & 5 & 6 \\
\hline
0 & 100.0 \cellcolor[rgb]{1.0, 0.67 , 0.67} & 83.629 \cellcolor[rgb]{1.0, 0.866 , 0.67} & 81.444 \cellcolor[rgb]{1.0, 0.893 , 0.67} & 82.891 \cellcolor[rgb]{1.0, 0.875 , 0.67} & 83.247 \cellcolor[rgb]{1.0, 0.871 , 0.67} & 72.117 \cellcolor[rgb]{0.995, 1.0 , 0.67} & 68.889 \cellcolor[rgb]{0.957, 1.0 , 0.67} \\
\hline
1 & 83.629 \cellcolor[rgb]{1.0, 0.866 , 0.67} & 100.0 \cellcolor[rgb]{1.0, 0.67 , 0.67} & 86.233 \cellcolor[rgb]{1.0, 0.835 , 0.67} & 86.367 \cellcolor[rgb]{1.0, 0.834 , 0.67} & 84.352 \cellcolor[rgb]{1.0, 0.858 , 0.67} & 67.481 \cellcolor[rgb]{0.94, 1.0 , 0.67} & 63.662 \cellcolor[rgb]{0.894, 1.0 , 0.67} \\
\hline
2 & 81.444 \cellcolor[rgb]{1.0, 0.893 , 0.67} & 86.233 \cellcolor[rgb]{1.0, 0.835 , 0.67} & 100.0 \cellcolor[rgb]{1.0, 0.67 , 0.67} & 86.357 \cellcolor[rgb]{1.0, 0.834 , 0.67} & 83.525 \cellcolor[rgb]{1.0, 0.868 , 0.67} & 65.476 \cellcolor[rgb]{0.916, 1.0 , 0.67} & 61.672 \cellcolor[rgb]{0.87, 1.0 , 0.67} \\
\hline
3 & 82.891 \cellcolor[rgb]{1.0, 0.875 , 0.67} & 86.367 \cellcolor[rgb]{1.0, 0.834 , 0.67} & 86.357 \cellcolor[rgb]{1.0, 0.834 , 0.67} & 100.0 \cellcolor[rgb]{1.0, 0.67 , 0.67} & 85.423 \cellcolor[rgb]{1.0, 0.845 , 0.67} & 67.436 \cellcolor[rgb]{0.939, 1.0 , 0.67} & 63.472 \cellcolor[rgb]{0.892, 1.0 , 0.67} \\
\hline
4 & 83.247 \cellcolor[rgb]{1.0, 0.871 , 0.67} & 84.352 \cellcolor[rgb]{1.0, 0.858 , 0.67} & 83.525 \cellcolor[rgb]{1.0, 0.868 , 0.67} & 85.423 \cellcolor[rgb]{1.0, 0.845 , 0.67} & 100.0 \cellcolor[rgb]{1.0, 0.67 , 0.67} & 70.398 \cellcolor[rgb]{0.975, 1.0 , 0.67} & 65.86 \cellcolor[rgb]{0.92, 1.0 , 0.67} \\
\hline
5 & 72.117 \cellcolor[rgb]{0.995, 1.0 , 0.67} & 67.481 \cellcolor[rgb]{0.94, 1.0 , 0.67} & 65.476 \cellcolor[rgb]{0.916, 1.0 , 0.67} & 67.436 \cellcolor[rgb]{0.939, 1.0 , 0.67} & 70.398 \cellcolor[rgb]{0.975, 1.0 , 0.67} & 100.0 \cellcolor[rgb]{1.0, 0.67 , 0.67} & 81.661 \cellcolor[rgb]{1.0, 0.89 , 0.67} \\
\hline
6 & 68.889 \cellcolor[rgb]{0.957, 1.0 , 0.67} & 63.662 \cellcolor[rgb]{0.894, 1.0 , 0.67} & 61.672 \cellcolor[rgb]{0.87, 1.0 , 0.67} & 63.472 \cellcolor[rgb]{0.892, 1.0 , 0.67} & 65.86 \cellcolor[rgb]{0.92, 1.0 , 0.67} & 81.661 \cellcolor[rgb]{1.0, 0.89 , 0.67} & 100.0 \cellcolor[rgb]{1.0, 0.67 , 0.67} \\
\hline
\end{tabular}
\end{center}
\end{table*}

\begin{table*}[htbp]
\caption{Facebook Friends}
\begin{center}
\begin{tabular}{|l|c|c|c|c|c|c|c|}
\hline
row & 0 & 1 & 2 & 3 & 4 & 5 & 6 \\
\hline
0 & 100.0 \cellcolor[rgb]{1.0, 0.67 , 0.67} & 86.873 \cellcolor[rgb]{1.0, 0.828 , 0.67} & 86.568 \cellcolor[rgb]{1.0, 0.831 , 0.67} & 86.321 \cellcolor[rgb]{1.0, 0.834 , 0.67} & 86.201 \cellcolor[rgb]{1.0, 0.836 , 0.67} & 83.52 \cellcolor[rgb]{1.0, 0.868 , 0.67} & 84.837 \cellcolor[rgb]{1.0, 0.852 , 0.67} \\
\hline
1 & 86.873 \cellcolor[rgb]{1.0, 0.828 , 0.67} & 100.0 \cellcolor[rgb]{1.0, 0.67 , 0.67} & 87.345 \cellcolor[rgb]{1.0, 0.822 , 0.67} & 87.098 \cellcolor[rgb]{1.0, 0.825 , 0.67} & 86.344 \cellcolor[rgb]{1.0, 0.834 , 0.67} & 81.782 \cellcolor[rgb]{1.0, 0.889 , 0.67} & 82.906 \cellcolor[rgb]{1.0, 0.875 , 0.67} \\
\hline
2 & 86.568 \cellcolor[rgb]{1.0, 0.831 , 0.67} & 87.345 \cellcolor[rgb]{1.0, 0.822 , 0.67} & 100.0 \cellcolor[rgb]{1.0, 0.67 , 0.67} & 87.35 \cellcolor[rgb]{1.0, 0.822 , 0.67} & 86.456 \cellcolor[rgb]{1.0, 0.833 , 0.67} & 81.663 \cellcolor[rgb]{1.0, 0.89 , 0.67} & 82.719 \cellcolor[rgb]{1.0, 0.877 , 0.67} \\
\hline
3 & 86.321 \cellcolor[rgb]{1.0, 0.834 , 0.67} & 87.098 \cellcolor[rgb]{1.0, 0.825 , 0.67} & 87.35 \cellcolor[rgb]{1.0, 0.822 , 0.67} & 100.0 \cellcolor[rgb]{1.0, 0.67 , 0.67} & 86.558 \cellcolor[rgb]{1.0, 0.831 , 0.67} & 81.303 \cellcolor[rgb]{1.0, 0.894 , 0.67} & 82.359 \cellcolor[rgb]{1.0, 0.882 , 0.67} \\
\hline
4 & 86.201 \cellcolor[rgb]{1.0, 0.836 , 0.67} & 86.344 \cellcolor[rgb]{1.0, 0.834 , 0.67} & 86.456 \cellcolor[rgb]{1.0, 0.833 , 0.67} & 86.558 \cellcolor[rgb]{1.0, 0.831 , 0.67} & 100.0 \cellcolor[rgb]{1.0, 0.67 , 0.67} & 83.293 \cellcolor[rgb]{1.0, 0.87 , 0.67} & 83.551 \cellcolor[rgb]{1.0, 0.867 , 0.67} \\
\hline
5 & 83.52 \cellcolor[rgb]{1.0, 0.868 , 0.67} & 81.782 \cellcolor[rgb]{1.0, 0.889 , 0.67} & 81.663 \cellcolor[rgb]{1.0, 0.89 , 0.67} & 81.303 \cellcolor[rgb]{1.0, 0.894 , 0.67} & 83.293 \cellcolor[rgb]{1.0, 0.87 , 0.67} & 100.0 \cellcolor[rgb]{1.0, 0.67 , 0.67} & 86.949 \cellcolor[rgb]{1.0, 0.827 , 0.67} \\
\hline
6 & 84.837 \cellcolor[rgb]{1.0, 0.852 , 0.67} & 82.906 \cellcolor[rgb]{1.0, 0.875 , 0.67} & 82.719 \cellcolor[rgb]{1.0, 0.877 , 0.67} & 82.359 \cellcolor[rgb]{1.0, 0.882 , 0.67} & 83.551 \cellcolor[rgb]{1.0, 0.867 , 0.67} & 86.949 \cellcolor[rgb]{1.0, 0.827 , 0.67} & 100.0 \cellcolor[rgb]{1.0, 0.67 , 0.67} \\
\hline
\end{tabular}
\end{center}
\end{table*}

\begin{table*}
    \captionsetup[table]{indention=0pt,margin=0pt,font=small}
    \tabcolsep=0.0cm
    \begin{tabular}{@{}cccc@{}}
      \multicolumn{4}{c} {
        \subcaptionbox{\label{fig:schedule_by_topic}}{\includegraphics[width=0.95\textwidth]{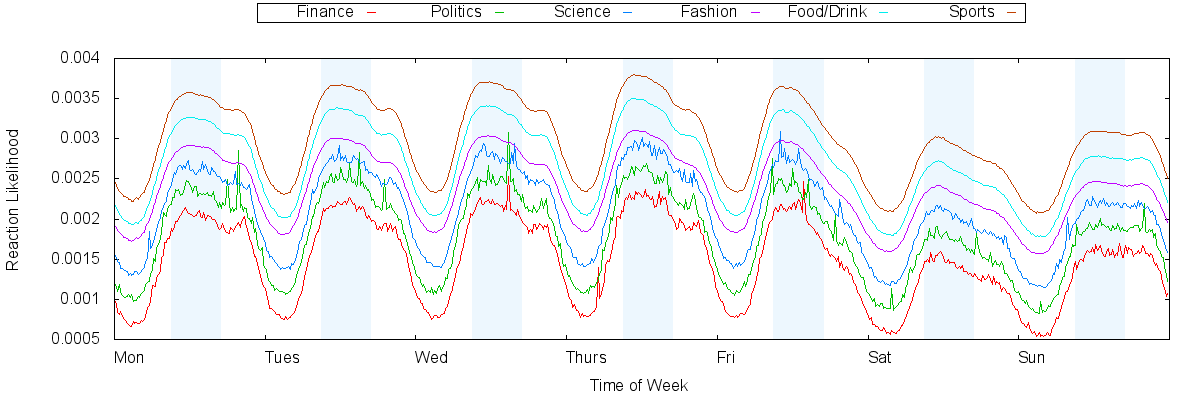}}
      } \\
      \subcaptionbox{\label{fig:same_topic_corrleation_fb}}{
        \includegraphics[height=1.6in]{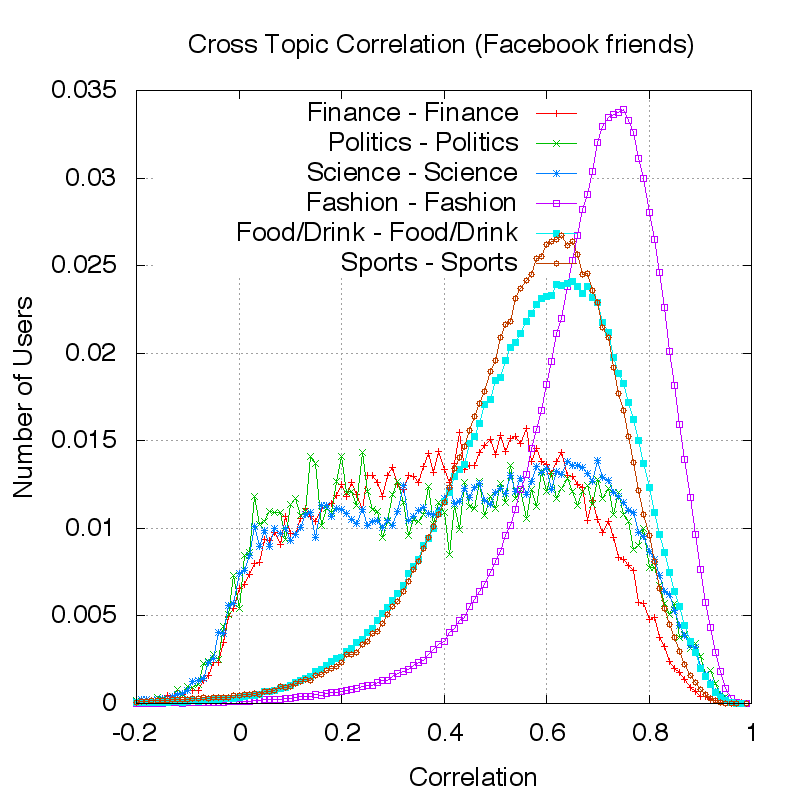}
      } &
      \subcaptionbox{\label{fig:same_topic_similarity_fb}}{
        \includegraphics[height=1.6in]{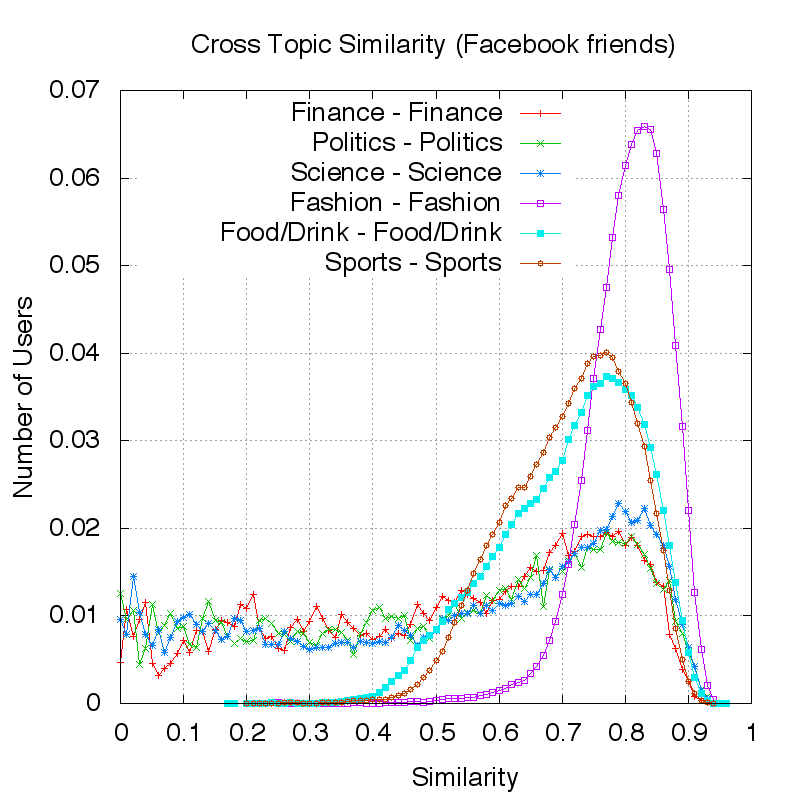}
      } &
      \subcaptionbox{\label{fig:cross_topic_corrleation_fb}}{
        \includegraphics[height=1.6in]{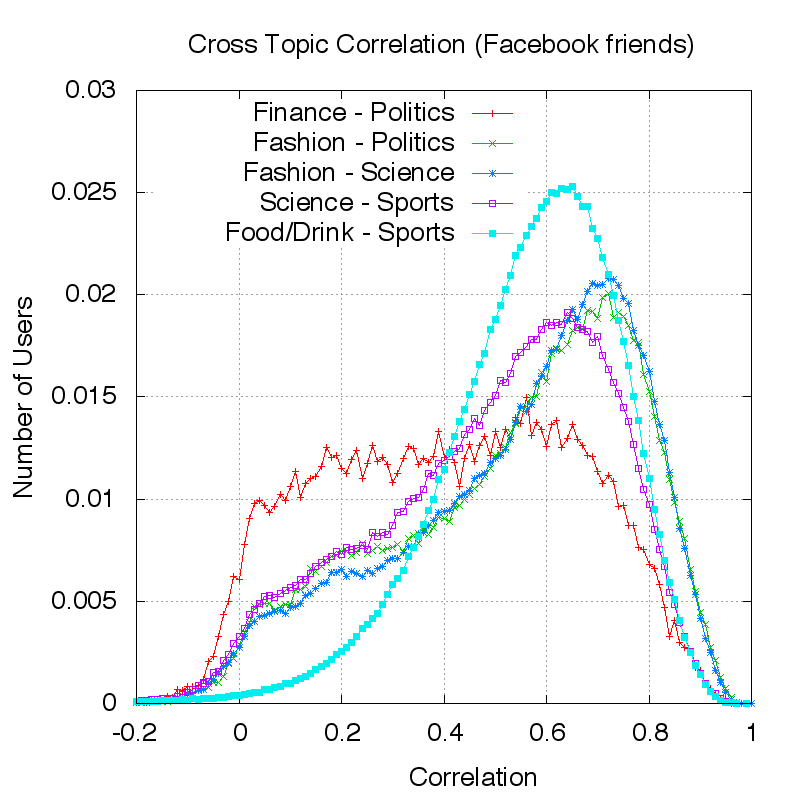}
      } &
      \subcaptionbox{\label{fig:cross_topic_similarity_fb}}{
        \includegraphics[height=1.6in]{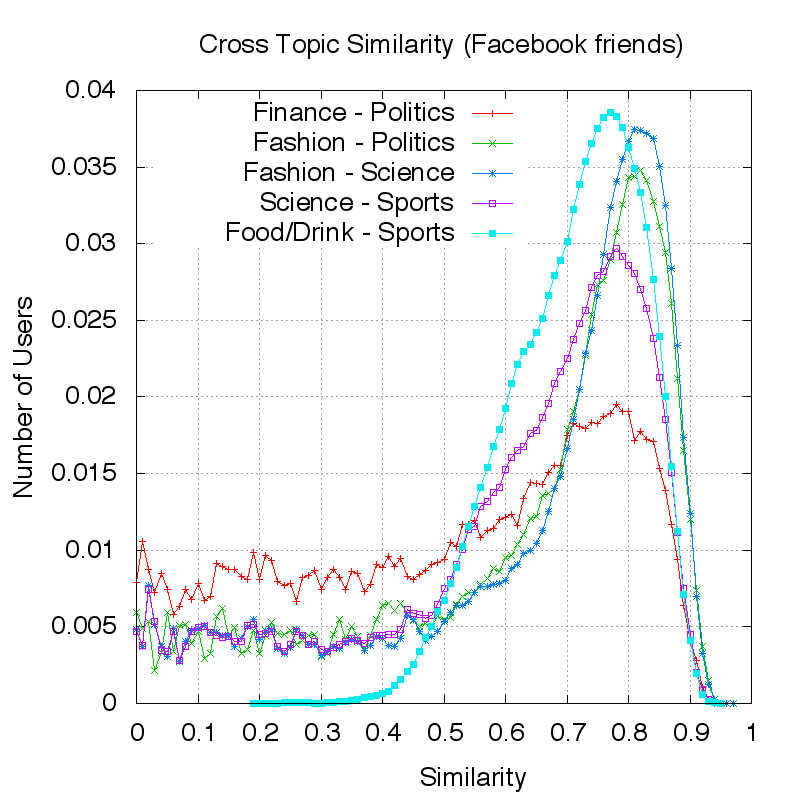}
      }
    \end{tabular}

    \caption{Analysis of aggregate topic (within NYC) level optimal post schedules for Facebook friends }
    \label{table:topic_analysis_table_fb}
\end{table*}

\begin{table*}
    \captionsetup[table]{indention=0pt,margin=0pt,font=small}
    \tabcolsep=0.0cm
    \begin{tabular}{@{}cccc@{}}
      \multicolumn{4}{c} {
        \subcaptionbox{\label{fig:schedule_by_topic}}{\includegraphics[width=0.95\textwidth]{schedule_by_topic/schedule_FB_FRIENDS}}
      } \\
      \subcaptionbox{\label{fig:same_topic_corrleation_tw}}{
        \includegraphics[height=1.6in]{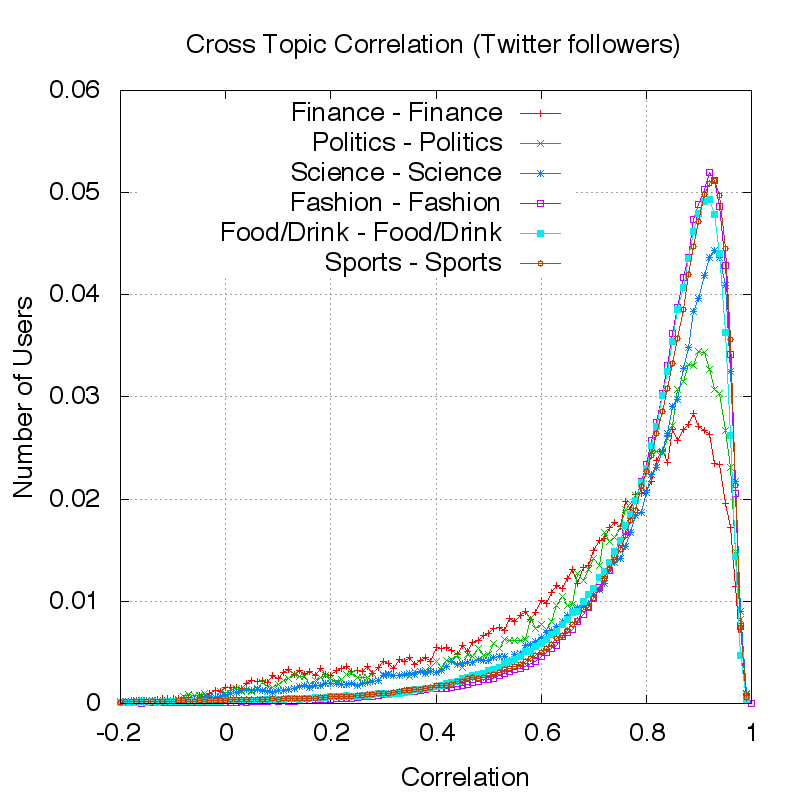}
      } &
      \subcaptionbox{\label{fig:same_topic_similarity_tw}}{
        \includegraphics[height=1.6in]{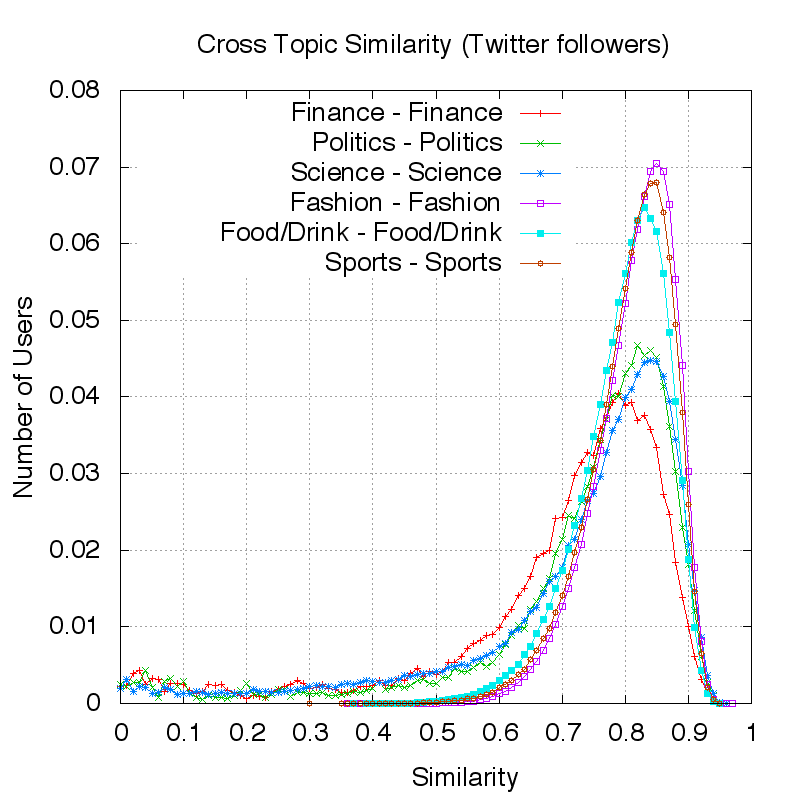}
      } &
      \subcaptionbox{\label{fig:cross_topic_corrleation_tw}}{
        \includegraphics[height=1.6in]{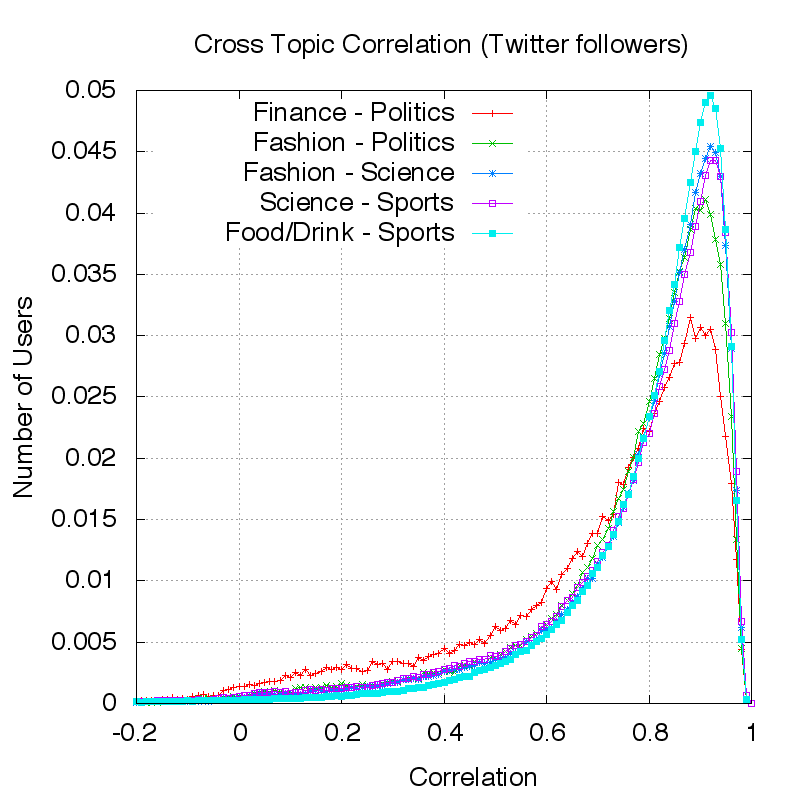}
      } &
      \subcaptionbox{\label{fig:cross_topic_similarity_tw}}{
        \includegraphics[height=1.6in]{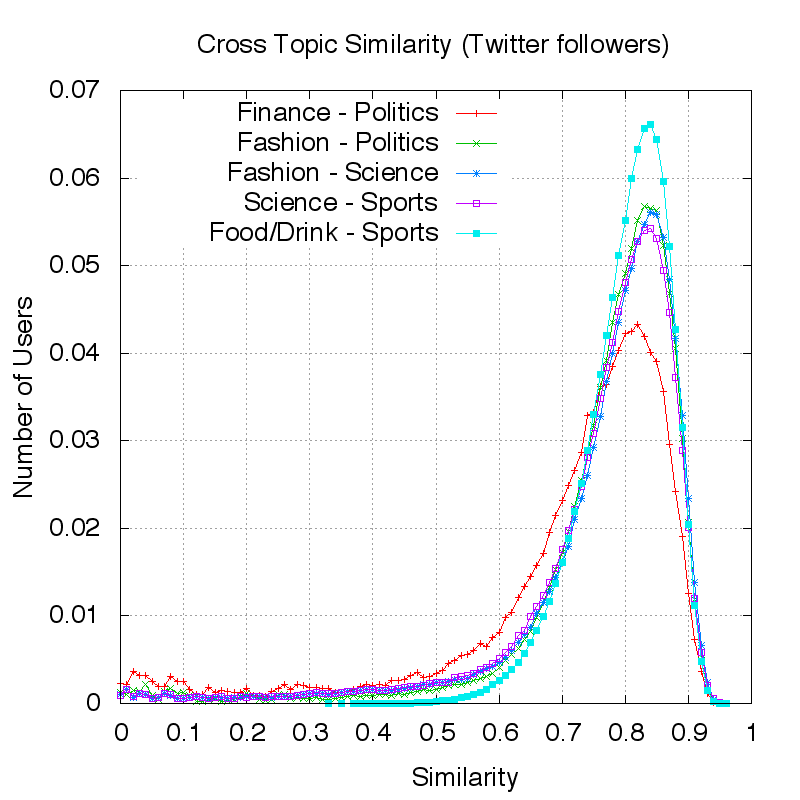}
      }
    \end{tabular}

    \caption{Analysis of aggregate topic (within NYC) level optimal post schedules for Twitter followers }
    \label{table:topic_analysis_table_tw}
\end{table*}

\begin{figure*}[htbp]
  \centering
  \fbox{\includegraphics[width=2.0\columnwidth]{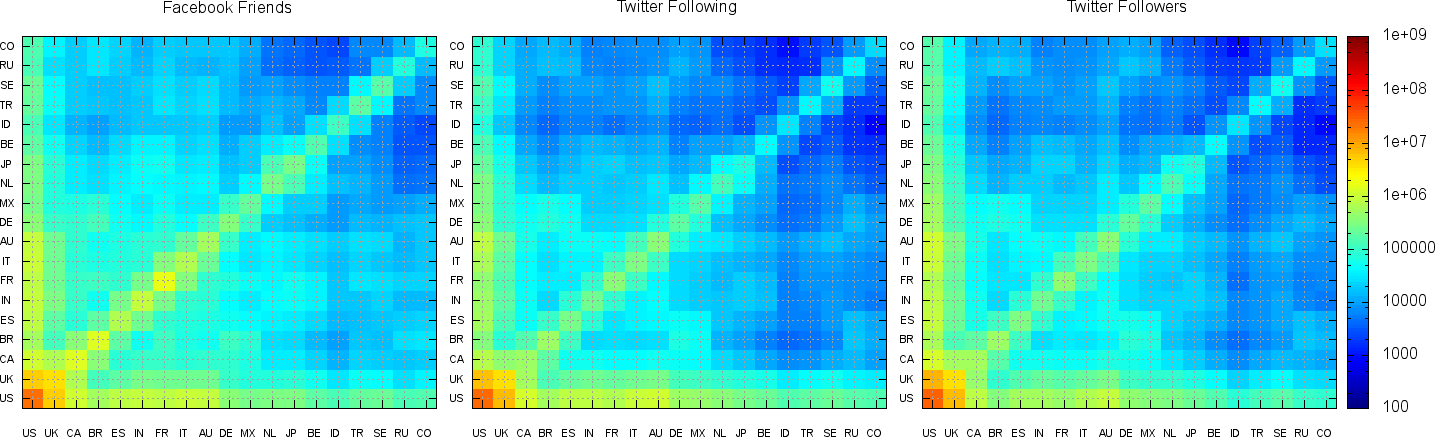}}
  \caption{Cross Country User Graph Correlation }
  \label{fig:cross_country_user_graph_correlation}
\end{figure*}

\begin{table*}[htbp]
\begin{center}
\caption{Optimal Times to Post for some Twitter Users}
\begin{tabular}{|c|c|c|c|c|c|c|c|} \hline
\multirow{2}{*}{User}
& \multirow{2}{*}{Monday} & \multirow{2}{*}{Tuesday} & \multirow{2}{*}{Wednesday} & \multirow{2}{*}{Thursday} & \multirow{2}{*}{Friday} & \multirow{2}{*}{Saturday} & \multirow{2}{*}{Sunday} \\ & & & & & & & \\ \hline
Barack Obama &\cellcolor{BlueGray}19:15-21:15 &\cellcolor{LightYellow}06:15-08:15 &\cellcolor{LightYellow}06:00-08:00 &\cellcolor{DarkGray}00:15-02:15 &\cellcolor{BlueGray}18:15-20:15 &\cellcolor{LightYellow}06:15-08:15 &\cellcolor{LightYellow}05:15-07:15\\ \cline{1-8}
Narendra Modi &\cellcolor{LightYellow}05:15-07:15 &\cellcolor{DarkGray}02:30-04:30 &\cellcolor{LightGray}03:00-05:00 &\cellcolor{BlueGray}21:45-23:45 &\cellcolor{LightYellow}05:15-07:15 &\cellcolor{DarkGray}01:00-03:00 &\cellcolor{LightBlue}15:30-17:30\\ \cline{1-8}
Bill Gates &\cellcolor{BrightestYellow}11:30-13:30 &\cellcolor{LightYellow}06:45-08:45 &\cellcolor{LightYellow}10:30-12:30 &\cellcolor{LightYellow}09:45-11:45 &\cellcolor{BlueGray}18:15-20:15 &\cellcolor{LightBlue}16:30-18:30 &\cellcolor{BlueGray}17:15-19:15\\ \cline{1-8}
Mark Cuban &\cellcolor{LightYellow}10:45-12:45 &\cellcolor{BrightestYellow}13:30-15:30 &\cellcolor{LightBlue}15:15-17:15 &\cellcolor{BrightestYellow}11:00-13:00 &\cellcolor{DarkGray}01:45-03:45 &\cellcolor{LightYellow}05:45-07:45 &\cellcolor{BlueGray}19:00-21:00\\ \cline{1-8}
Britney Spears &\cellcolor{BlueGray}21:45-23:45 &\cellcolor{BlueGray}21:45-23:45 &\cellcolor{BlueGray}21:00-23:00 &\cellcolor{DarkGray}00:00-02:00 &\cellcolor{DarkGray}00:30-02:30 &\cellcolor{LightGray}04:00-06:00 &\cellcolor{BrightestYellow}13:15-15:15\\ \cline{1-8}
Lil Wayne &\cellcolor{DarkGray}02:45-04:45 &\cellcolor{BrightestYellow}13:00-15:00 &\cellcolor{DarkGray}01:45-03:45 &\cellcolor{LightYellow}10:15-12:15 &\cellcolor{BlueGray}19:30-21:30 &\cellcolor{LightYellow}09:30-11:30 &\cellcolor{BrightestYellow}13:15-15:15\\ \cline{1-8}
Justin Timberlake  &\cellcolor{BlueGray}19:45-21:45 &\cellcolor{BlueGray}20:00-22:00 &\cellcolor{BlueGray}20:30-22:30 &\cellcolor{LightBlue}16:00-18:00 &\cellcolor{LightBlue}15:45-17:45 &\cellcolor{BrightestYellow}11:00-13:00 &\cellcolor{BrightestYellow}13:45-15:45\\ \cline{1-8}
Marc Andreessen &\cellcolor{BrightestYellow}11:00-13:00 &\cellcolor{LightYellow}05:45-07:45 &\cellcolor{LightYellow}09:30-11:30 &\cellcolor{BlueGray}21:45-23:45 &\cellcolor{LightYellow}10:45-12:45 &\cellcolor{BlueGray}21:15-23:15 &\cellcolor{BlueGray}21:00-23:00\\ \cline{1-8}
Robert Scoble &\cellcolor{BlueGray}21:45-23:45 &\cellcolor{LightYellow}05:15-07:15 &\cellcolor{BlueGray}21:45-23:45 &\cellcolor{BlueGray}21:45-23:45 &\cellcolor{LightYellow}07:30-09:30 &\cellcolor{BlueGray}21:30-23:30 &\cellcolor{BlueGray}21:00-23:00\\ \cline{1-8}
Guy Kawasaki &\cellcolor{LightGray}03:30-05:30 &\cellcolor{DarkGray}02:45-04:45 &\cellcolor{DarkGray}01:15-03:15 &\cellcolor{DarkGray}02:00-04:00 &\cellcolor{LightGray}03:30-05:30 &\cellcolor{LightBlue}15:45-17:45 &\cellcolor{LightBlue}16:00-18:00\\ \cline{1-8}
Red Bull &\cellcolor{BlueGray}21:45-23:45 &\cellcolor{LightYellow}06:45-08:45 &\cellcolor{BlueGray}21:45-23:45 &\cellcolor{DarkGray}00:00-02:00 &\cellcolor{LightYellow}07:45-09:45 &\cellcolor{DarkGray}01:00-03:00 &\cellcolor{LightYellow}09:15-11:15\\ \cline{1-8}
Coca-Cola  &\cellcolor{BlueGray}21:45-23:45 &\cellcolor{BlueGray}21:45-23:45 &\cellcolor{BlueGray}21:00-23:00 &\cellcolor{BlueGray}21:15-23:15 &\cellcolor{BlueGray}21:45-23:45 &\cellcolor{BlueGray}21:30-23:30 &\cellcolor{BlueGray}21:00-23:00\\ \cline{1-8}
BuzzFeed &\cellcolor{BrightestYellow}12:15-14:15 &\cellcolor{BlueGray}18:45-20:45 &\cellcolor{BrightestYellow}12:30-14:30 &\cellcolor{BrightestYellow}13:15-15:15 &\cellcolor{BrightestYellow}11:45-13:45 &\cellcolor{BrightestYellow}14:45-16:45 &\cellcolor{BlueGray}21:30-23:30\\ \cline{1-8}
San Francisco Giants  &\cellcolor{BlueGray}21:30-23:30 &\cellcolor{BlueGray}21:00-23:00 &\cellcolor{BlueGray}21:30-23:30 &\cellcolor{BlueGray}21:45-23:45 &\cellcolor{DarkGray}00:00-02:00 &\cellcolor{BlueGray}20:45-22:45 &\cellcolor{BlueGray}21:15-23:15\\ \cline{1-8}
NFL Network &\cellcolor{LightYellow}06:45-08:45 &\cellcolor{BlueGray}18:15-20:15 &\cellcolor{LightYellow}06:15-08:15 &\cellcolor{LightYellow}06:30-08:30 &\cellcolor{BrightestYellow}12:30-14:30 &\cellcolor{BrightestYellow}14:15-16:15 &\cellcolor{LightYellow}07:30-09:30\\ \cline{1-8}
Liverpool FC &\cellcolor{BlueGray}17:30-19:30 &\cellcolor{BlueGray}18:15-20:15 &\cellcolor{BlueGray}19:15-21:15 &\cellcolor{BlueGray}19:45-21:45 &\cellcolor{BlueGray}20:00-22:00 &\cellcolor{BlueGray}20:30-22:30 &\cellcolor{BlueGray}20:30-22:30\\ \cline{1-8}
Real Madrid &\cellcolor{LightYellow}10:00-12:00 &\cellcolor{LightYellow}09:45-11:45 &\cellcolor{LightYellow}09:00-11:00 &\cellcolor{LightYellow}10:30-12:30 &\cellcolor{LightYellow}08:00-10:00 &\cellcolor{BlueGray}20:00-22:00 &\cellcolor{LightYellow}09:45-11:45\\ \cline{1-8}
Boston Red Sox &\cellcolor{LightYellow}06:15-08:15 &\cellcolor{LightYellow}06:00-08:00 &\cellcolor{LightYellow}06:45-08:45 &\cellcolor{BrightestYellow}14:00-16:00 &\cellcolor{LightYellow}07:45-09:45 &\cellcolor{LightYellow}05:30-07:30 &\cellcolor{LightYellow}08:45-10:45\\ \cline{1-8}
\end{tabular}
\end{center}
\end{table*}
